# Supplementary material for: The Medkit-Learn(ing) Environment: Medical Decision Modelling through Simulation
Source: arXiv:2106.04240 source file (2022-03-14)
Supplement: Supplementary file 1 [file appendix.tex]

\appendix

\parfillskip=0pt plus 1fil

\textbf{Python Repo:} \url{https://github.com/XanderJC/medkit-learn}

\section{Domains and Real Data Information}

\subsection{Hospital Wards.}
The \emph{Ward} domain is based on the care of 6,321 patients at the Ronald Reagan UCLA Medical Center in California who were treated on the general medicine floor between 2013-2016 \citeApp{alaa2017personalized}. These patients were treated for a variety of conditions including pneumonia, sepsis, and fevers were in general stable and deterioration that required ICU care was rare. Measurements were taken roughly every 4 hours, with average stays lasting 9 days, and include common vital signs such as pulse and blood pressure alongside lab tests and results and include 8 static (although categorical features are one-hot encoded, extending the space) and 35 temporal features for which we model the dynamics. The action space is taken as a choice of one to three binary actions (encoded for a maximum size of eight) marking the treatment of various oxygen therapy devices. 

\subsection{Intensive Care Unit.}
The \emph{ICU} domain simulates the treatment of 23,106 of patients in the intensive care unit from Amsterdam UMC \citeApp{elbers2019amsterdam}. These patients are in a more critical state than those on the general wards while suffering similarly from a variety of conditions and consequently are monitored more frequently, with the database containing around 1 billion clinical observations at varying timesteps down to minute by minute recordings. We aggregate data into one hour timesteps and model the treatment of mechanical ventilation alongside the prescription of antibiotics and oxygentherapy. We include 36 static features including height, initial weight, and commorbidities with 24 series features focusing on vital signs including heart rate, blood pressure, and various chemical blood concentration levels.

\section{Further Environment Model Details}

\subsection{The Customised State Space Model}

The CSS is a variety of a deep non-Markovian hidden state-space model. 
The \emph{non-Markovianity} comes from the property in the model that transitions are parameterised given discrete states simply as follows:
\begin{small}
\begin{align}
    p(z_t|\vec{x}_{t-1},\vec{y}_{t-1},\vec{z}_{t-1}) &= p(z_t|\vec{\alpha}_{t},\vec{z}_{t-1}) \nonumber \\
    &= \sum_{t'=1}^{t-1} \alpha_{t'}^{t-1}\mathbf{P}_{y_{t'}}(z_{t'},z_t),
\end{align}
\end{small}
with $\mathbf{P}_{y_t}$ a baseline transition matrix given intervention $y_t$ is made and $\alpha_{t'}^{t-1}$ some attention weight on the previous timesteps such that $\sum_{t'=1}^{t-1} \alpha_{t'}^{t-1} = 1$. This departs from the traditional IOHMM \citepApp{bengio1995input} by the inclusion of the attention weights that induce time-dependency on points further in the past than the previous time point and can be learnt during training.

The emission distribution allows for a flexible representation: let $p_\psi(x_t)$ be any distribution with support over $\mathcal{X}$ and parameter(s) $\psi$ (for example some Gaussian mixture) then we let:
\begin{align}
    p(x_t|z_t,x_s) = p_{\psi^*}(x_t), \quad \text{with} \;\psi^* = f_\gamma(z_t,x_s).
\end{align}
We take $f_\gamma$ to be a $\gamma$-parameterised function approximator to output the parameters of the emission distribution given the current state and static features of the patient - a standard choice being an MLP that takes in the concatenation of $z_t$ and $x_s$. This alleviates a common problem with state-space models where the observations are ultimately drawn from some finite mixture of distributions of order $|\mathcal{Z}|$, as now the dependence on the static features allows for a very flexible output. The CSS dynamics model allows Medkit users to post-hoc customise the number of states and the Markovianity of the environment through the attention mechanism (e.g users can pass a vector that specifies exact weights or an integer representing the number of states back to look.)

\paragraph{Learning and inference.}
Exact inference over the hidden states in this model is intractable and so we use an inference network to parameterise an approximate posterior over the latent hidden state, in particular assuming a factorisation that mirrors the true structure of the posterior as follows:
\begin{align}
    q_\phi(\vec{z}_T|\vec{x}_T,\vec{y}_{T}) &= q_\phi(z_1|\vec{x}_T,\vec{y}_{T})  \prod_{t=2}^T q_\phi(z_t|z_{t-1},\vec{x}_{t:T},\vec{y}_{t:T}).
\end{align}
Thus the posterior depends on the previous hidden state and all future observations and actions. This can be practically achieved by using a backward LSTM \citepApp{hochreiter1997long} to summarise the future into its hidden state before passing that and the previous state into a new network to obtain the approximate posterior.

Our inference network leads to a factorised Evidence Lower BOund (ELBO) given by:

\begin{align}
    \log p_\theta(\vec{x}_T|\vec{y}_{T-1}) &\geq \mathbb{E}_{q_\phi} \big[ \log p_\theta(\vec{x}_T,\vec{z}_T|\vec{y}_{T-1})  - \log q_\phi(\vec{z}_T|\vec{x}_T,\vec{y}_{T}) \big], 
\end{align}

leading to an optimisation task over $\theta$ and $\phi$. This is readily done using stochastic variational inference whereby we take a Monte Carlo estimate of the ELBO by sampling from the posterior and taking gradients \citeApp{krishnan2017structured}.

\subsection{The Sequential VAE Model}

The SVAE is again a variety of a deep non-Markovian hidden state-space model, although now the states are no longer discrete but rather live in some latent space of $\mathbb{R}^d$.
This then allows for more flexibility in the transition dynamics, in particular by making use of neural architectures. An encoder network predicts the approximate posterior over the latent variables and we employ essentially the same method as for teacher forcing in order to model dynamics in the latent space.
This again means that an inference network is required for doing approximate inference and similarly leads to an ELBO optimisation scheme.
With a joint optimisation scheme, we learn a representation that generates the observations well but also captures the features relevant for the transitions. This expressiveness allows for a higher fidelity model than the custom state-space but however comes at the cost of interpretable structure which we have established may be useful should algorithms be designed to uncover such things.

\section {Further Experimental Details}

\subsection{Computation}

All experiments were performed on a 2016 MacBook Pro, using a 2.9 GHz Dual-Core Intel Core i5 with 8GB of LPDDR3 RAM and no GPU acceleration.

\subsection{Predictive Score}

The predictive score measures how well the synthetic data can be used as a direct substitute for real data when it comes to a prediction task. 

For our experiments we generate 500 sample trajectories of maximum length 30 to be used as the synthetic data. A network consisting of an LSTM layer followed by two fully connected layers is then trained on this data for 50 epochs. This is then applied to a real data set and the AUROC is reported.

\subsection{Discriminative Score}

The discriminative score measures how well the synthetic data `hides' amongst real data.

For our experiments a training dataset is generated using 100 real trajectories and 100 synthetic trajectories along with their associated real/synthetic label. A single layer LSTM is then trained on this dataset to predict the label, before being applied to a test set of 100 real trajectories and 100 synthetic trajectories. We report the absolute value of the test accuracy minus 0.5.

\subsection{Imitation Learning Benchmarks}

All methods used are based on neural network and so in the experiments we maintain the same architecture of 2 hidden layers of 64 units each connected by exponential linear unit (ELU) activation functions.

Publicly available code was used in the implementations of a number of the benchmarks, specifically:

\begin{itemize}
    \item VDICE \citeApp{kostrikov2019imitation}:\\ \url{https://github.com/google-research/google-research/tree/master/value_dice} \\
    \item EDM \citeApp{jarrett2020strictly}:\\ \url{https://github.com/wgrathwohl/JEM}
\end{itemize}

Note that VDICE was originally designed for continuous actions with a Normal distribution output which we adapt for the experiments by replacing with a Gumbel-softmax.

\section{Frequently Asked Questions}

\textbf{Q: What would the process be for outside contributors wanting to add new medical domains?}

\textbf{A:} This should be relatively easy. The first way would be for them to provide us with a copy of the medical data, we could then add the details and train the models before adding them to the package. If they would rather not share the data, then the second way would be for the outside contributors themselves to fork the repo, define the domain, and train the models using the codebase before making a pull request to us. We would then make sure the pre-trained models work appropriately before merging into the package.

\textbf{Q: Could Medkit not generate biased or inappropriately skewed data?}

\textbf{A:} It is definitely possible, as with any generative model, however, we have inspected all of the models to try to ensure that this is not happening. We would emphasize that the data generated by Medkit should not be used for scientific discovery though - for example, it should not be used to say anything about how real doctors treat patients in the ICU nor how real patients will react to treatment. It is rather intended to be used with a focus on inspecting algorithms for decision modelling.

\textbf{Q: How important is the use of differential privacy in the training of the models?} 

\textbf{A:} We would like to emphasize that all of the real data used to train models within Medkit had already undergone a full pre-processing procedure from their respective data guardians to de-identify the data and ensure the privacy of individuals. As a consequence, the added differential privacy layer that we add is not essential but does serve as an extra “insurance policy” just in case.

\textbf{Q: Can Medkit be used effectively for traditional model based reinforcement learning?}

\textbf{A:} It is worth saying that model-based RL is certainly not the focus of this work, as we’re much more interested in decision modelling based on the policy of a demonstrator. There are no prescribed rewards in Medkit at the moment - so agents cannot be trained out-of-the-box, however a reward function can be manually specified and integrated if the user so wishes.

\bibliographyApp{references}
\bibliographystyleApp{apalike}
